# Supplementary material for: High quality beam produced by tightly focused laser driven wakefield accelerators
Source: arXiv:2304.10730 source file (2023-04-21)
Supplement: Supplementary file 1 [file tight_focus_injection_supplementary_material.pdf]

# Supplemental Material: obtaining the empirical expression for $\Gamma$

Jia Wang, Ming Zeng, Dazhang Li, Xiaoning Wang, Jie Gao

April 20, 2023

The parameter $\Gamma$ is essential for predicting charge. We assume $\Gamma$ linearly depends on $n_p$, $a_0$ and $w_0$ within a certain parameter space, which can be written as

$$\Gamma = \frac{n_p}{C_n} + \frac{a_0}{C_a} + \frac{w_0}{C_w} + \Gamma_0, \tag{1}$$

where $C_n$, $C_a$, $C_w$ and $\Gamma_0$ are constants. Through a series of PIC simulations as shown in Fig.1, we get the following empirical formula in the parameter space $5 \leq a_0 \leq 20$, $2\ \mu\text{m} < w_0 \leq 10\ \mu\text{m}$ and $n_p \sim 10^{18}\ \text{cm}^{-3}$

$$\Gamma \approx -\frac{n_p\left[10^{18}\ \text{cm}^{-3}\right]}{20.16} + \frac{a_0}{100} - \frac{w_0\,[\mu\text{m}]}{46.42} + 1.029. \tag{2}$$

One may notice that Eq. (2) does not exactly predict all the lines in Fig.1. The constants in Eq. (2) are actually obtained by fitting the curves.

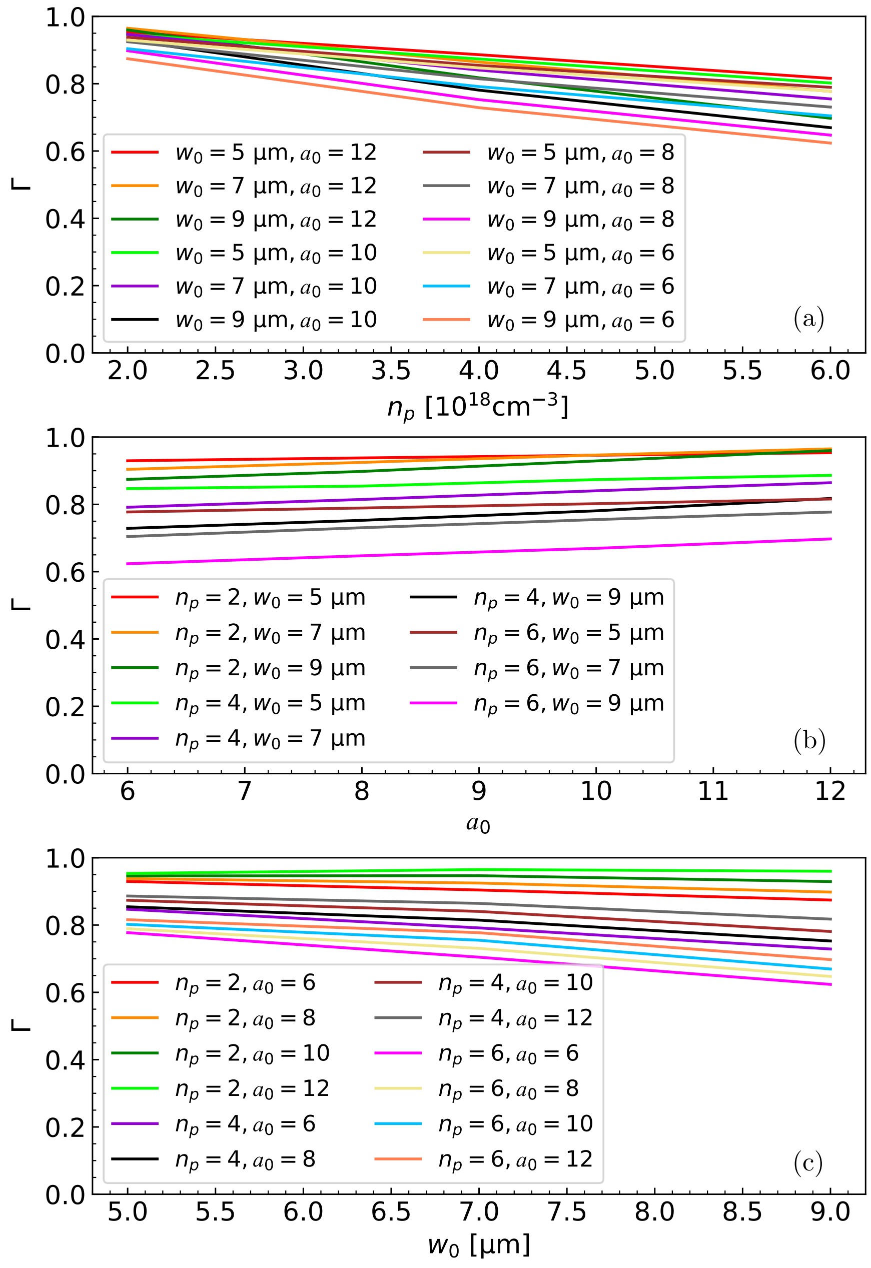


Figure 1: The dependecies of $\Gamma$ on $n_p$ (a), $a_0$ (b) and $w_0$ (c). The values of $n_p$ have the unit of $10^{18}$ cm$^{-3}$. The laser focal position $z_f$ is fixed at $z = 200$ $\mu$m and the laser wavelength $\lambda$ is fixed at 800 nm.
